# Supplementary material for: A Light-Hole Quantum Well on Silicon
Source: arXiv:2112.15185 ancillary file (2022-01-03)
Supplement: Supplementary file 1 [file LH_QW_SI.pdf]

# Supplementary Information

# A Light-Hole Quantum Well on Silicon

Simone Assali,[1,*] Anis Attiaoui,[1,*] Patrick Del Vecchio,[1,*] Samik Mukherjee,[1] Jérôme Nicolas,[1] and Oussama Moutanabbir[1,**]

[1]Department of Engineering Physics, École Polytechnique de Montréal, C. P. 6079, Succ. Centre-Ville, Montréal, Québec H3C 3A7, Canada

Contents

**S1. XRD Characterization** ........ 2

S1.1. *Evaluation of Sn content and epitaxial strain from RSM maps* ........ 2

S1.2. *Estimation of the tensile strained Ge QW* ........ 2

**S2. Optical Modelling Methodology** ........ 5

S2.1. *p-doped Silicon Substrate* ........ 5

S2.2. *Ge-Virtual Substrate (Ge-VS)* ........ 6

S2.3. *Optical Modeling Strategy* ........ 7

**S3. Structural and optical characterization of s-Ge QWs** ........ 10

S3.1. *Ge QW at 1.1% tensile strain* ........ 10

S3.2. *Uncapped Ge layer at 1.1% tensile strain* ........ 10

S3.3. *Ge QW at 1.65% tensile strain* ........ 12

**S4. Theoretical Simulation** ........ 16

S4.1. *Eight-band* $\boldsymbol{k\cdot p}$ *GeSn Parametrization* ........ 16

S4.2. *Magnetic Field incorporation in Eight-band* $\boldsymbol{k\cdot p}$ ........ 17

S4.3. *Light hole-heavy hole mixing in highly tensile strained Ge QWs* ........ 17

**S5. References** ........ 20

## S1. XRD Characterization

S1.1. *Evaluation of Sn content and epitaxial strain from RSM maps*

To estimate the Sn composition in as-grown $Ge_{1-x}Sn_x$ epitaxial layers, the following analysis was carried out. First, the experimental in-plane $a_{\parallel}$ and out-of-plane lattice $a_{\perp}$ are calculated according to:

$$a_{\parallel} = \frac{\sqrt{h^2 + k^2}}{q_x};\ a_{\perp} = \frac{l}{q_z} \tag{1.1}$$

where $h$, $k$ and $l$ are the Miller indices of the diffracting (hkl) plane and $q_x$ and $q_z$ are the coordinates of the diffraction peak extracted from the reciprocal space map (RSM). These values are used to compute the unstrained lattice parameter using the following relationships:

$$a_0 = \frac{a_{\perp} + \frac{2C_{12}}{C_{11}} a_{\parallel}}{1 + \frac{2C_{12}}{C_{11}}} \tag{1.2}$$

$$\frac{C_{12}}{C_{11}} = 0.37492 - 3.69\,.\,10^{-6}\,T + 0.1676x - 0.0296x^2 \tag{1.3}$$

where $C_{11}$ and $C_{12}$ are the second order elastic moduli of the $Ge_{1-x}Sn_x$ material. The value of the $C_{12}/C_{11}$ ratio varies with the Sn content and is estimated using the formula proposed by Xu et Menéndez.[1–3] Finally, the Sn content can be found from the original lattice parameter via the Vegard's law:

$$a_0 = x.a_{Sn} + (1-x).a_{Ge} + x.(1-x).b_{GeSn} \tag{1.4}$$

in which $x$ is the Sn concentration in the GeSn alloy and $a_0$, $a_{Sn}$ and $a_{Ge}$ are the unstrained lattice parameters of $Ge_{1-x}Sn_x$, Sn, and Ge, respectively. $b_{GeSn}$ is the lattice bowing parameter. We use $b_{GeSn} = -0.041$ Å determined experimentally by Gencarelli et *al.* [4] The last step is to solve equation (1.4) for $x$ to find the concentration of Sn and the epitaxial strain in the $Ge_{1-x}Sn_x$ alloy.

S1.2. *Estimation of the tensile strained Ge QW*

The effect of the coherent s-Ge layer growth on the GeSn layers is visible in the XRD (004) symmetric scan in Fig. S1a. In the reference sample without the s-Ge layer (red curve) the GeSn-

related peaks are observed between 64.2° and 65.5°, with the TL and BR peaks being both at 64.25°. When the 12.5 nm-thick s-Ge layer is introduced in the stacking, the BR peak shifts to 64.0° while the TL peak remains at ~64.25° (blue curve). In addition, Pendellosung fringes are observed below 64.0°, which originate from the phase shift between the scattered waves induced by the variation in the out-of-plane lattice parameter across the BR/s-Ge/TL stacking.[5,6] As the interference fringes are only observed if a coherent epitaxy is present across the heterostructure, this further indicates the pseudomorphic nature of the s-Ge layer. We note that due to the limited number of fringes (2x) in the XRD scan a precise fit of the data using the dynamical simulation is rather cumbersome. Nonetheless, a tensile strain in the Ge QW higher than 1 % is indicated by the dynamical simulation, which lies in the same range as the value estimated from the RSM measurements discussed below (Fig. S1b). No clear peak associated with the strained Ge layer is visible in the (004) scan (Fig. S1a). The XRD peak for bulk Ge would be observed at 66.0°, while any tensile strain would shift the peak to larger angles, as observed for the tensile strain of 0.16 % in the Ge-VS that results in a peak at 66.06°. Tensile-strained Ge layers with a thickness of 15-30 nm and strain up to ~2 % grown on a $In_xGa_{1-x}As$/GaAs VS showed a weak XRD shoulder peak in the 66.4-67.0° range.[7,8] The contribution of the strained Ge peak was not observed in the (004) scan in Fig. S1a, most likely due to the small thickness of the layer (≤13 nm) in combination with the broader residual signal of the Ge-VS compared to a bulk GaAs wafer, which makes it more difficult to decouple the two signal contributions. However, we highlight that the presence of Pendellosung fringes (BR) in the present work indicates a higher crystallinity in the heterostructure compared to the previously shown hybrid group IV/III-V heterostructures. Due to the coherent growth of the s-Ge layer as demonstrated by the HRSTEM analysis (Figs. 2 and 4), the RSM peak for the s-Ge is expected with the same $q_x$=4.945±0.050 nm$^{-1}$ value of the TL, BR layers (dashed white vertical line in panel b and c of Fig. S1). However, due to the very small thickness of the s-Ge layer, estimating its signal in the RSM map is challenging, as it partially overwhelmed by the Ge-VS broad peak, as already discussed. By comparing high resolution RSM maps of the Ge-VS peak region with a sample grown without the s-Ge layer (Fig. S1d), a broadening of the Ge-related peak is observed (Fig. S1c), showing a maximum intensity in correspondence of $q_x$ value of the TL and BR layers, as expected for pseudomorphic s-Ge growth to these layers. From the RSM map an in-plane lattice $a_{\|}$= 5.720±0.050 Å is estimated for the s-Ge layer, which results in an in-plane tensile strain $\varepsilon_{\|}$=1.1±0.1 %. Since a precise value for the $q_z$ for the s-Ge peak cannot be

$_{\perp}$ cannot be determined. To that end, synchrotron measurement was undertaken to better quantify the $q_z$ value (to be reported elsewhere).

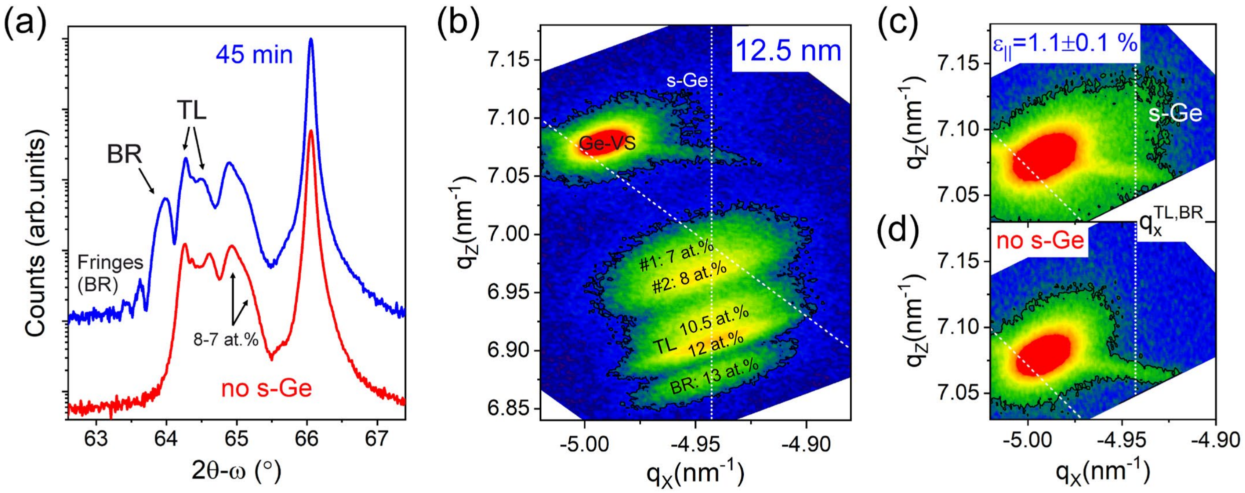


Figure S1: (a) 2θ-ω scans around the (004) X-ray diffraction order for the 12.5 nm-thick QW (blue curve) and the reference stacking without s-Ge well (red curve). (b) RSM around the asymmetrical (224) reflection for the 12.5 nm-thick QW. (c-d) HRRSM maps acquired in the Ge-VS peak region showing the presence of the s-Ge peak when compared to the reference stacking without strained Ge growth.

**S2. Optical Modelling Methodology**

S2.1. *p-doped Silicon Substrate*

Infrared spectroscopic ellipsometry (IRSE) provide the possibility to obtain quantitatively the free-electron contribution in the range of screened plasma energy, leading to a consistent description of the most pronounced infrared optical effects in doped substrate. The Boron-doped silicon substrate wafer (with a resistivity $\rho$ between 1 and 10 $\Omega.cm$) was characterized with the IRSE at 4 angles of incidence (AOI) ranging from 72° to 78° with 2° step. The spectral resolution was set to 8 $cm^{-1}$. To obtain sufficient signal to noise ratio for the weak spectral structure studied, the spectra were heavily accumulated. All measurements were performed at room temperature. The SE parameter $(Tan\,\Psi)$ is plotted in Fig. S2 against the photon energy for two AOI together with the best-fit lineshapes (red-dashed lines) based upon a simple Drude Model, where the real $\varepsilon_1$ and imaginary $\varepsilon_2$ dielectric function are defined as

$$\varepsilon_1 = \varepsilon_\infty \left[1 - \frac{\omega_p^2}{\omega_\tau^2(1+\omega^2/\omega_\tau^2)}\right] \; and \; \varepsilon_2 = \frac{\varepsilon_\infty \omega_p^2}{\omega_\tau \omega(1+\omega^2/\omega_\tau^2)}$$

where $\varepsilon_\infty$ is the high frequency dielectric constant at frequencies well above the bulk plasma frequency $\omega_p$. The relaxation frequency $\omega_\tau = 1/\tau$ where $\tau$ is the relaxation time.

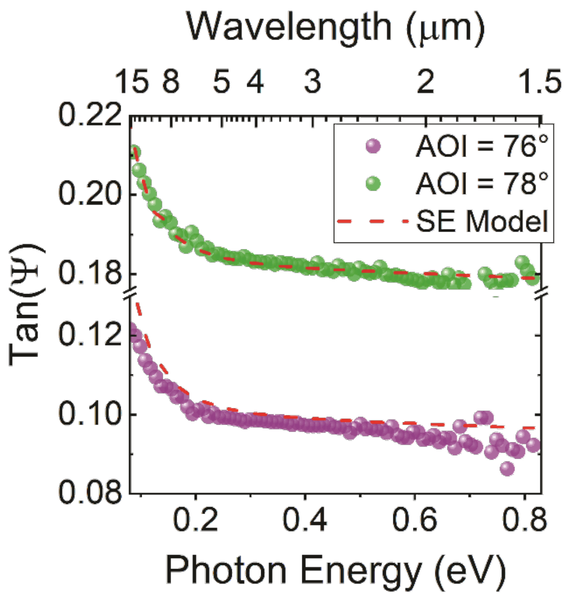

An additional consistency check of the built optical model is to compare the extracted resistivity from the Drude model to the real value of the Si substrate wafer. The current measurement yielded a resistivity of 4.65 $\Omega.cm$, which falls within the range of the manufacturer resistivity.

S2.2. *Ge-Virtual Substrate (Ge-VS)*

Spectroscopic ellipsometry and absorbance measurement were combined to evaluate the dielectric function of the Ge-VS. It has been already established that the sensitivity of SE is always enhanced close to the Brewster angle. The Brewster angle of Ge is 78.2°. Furthermore, Differential absorbance measurement highlight the presence of two interband transition related to the Ge direct band gap between $\Gamma - LH$ and $\Gamma - HH$. The measurement is corroborated with 8-band $k.p$ simulations where the effect of tensile strain on the direct gap transitions in Ge-VS is accounted for through the Bir-Pikus formalism. The strain in the epitaxial Ge films was measured by acquiring the Ge (400) symmetric high resolution Xray diffraction (HRXRD) step scan and was found to be tensile strained with a value of 0.13%. Fig S3a present the XRD step scan for the tensile Ge-VS layer where the blue and red arrows highlight respectively the theoretical position (θ=32.997°) of a relaxed Ge layer and the measured CVD-grown 950 nm tensile strained (θ=33.045°) Ge layer. Additionally, Fig S3b show the absorbance measurement of the Ge-VS sample. The interference fringes indicate a Ge layer of 948.5 nm, which is consolidated with IRSE modelling. Furthermore, the derivative of the absorbance spectra shows the presence of two interband transition peaks in the energy range of 0.75 and 0.85 eV. The exact peak positions are estimated by fitting the direct gap transition with 2 Gaussians peak functions, as shown in Fig. S3c. The $\Gamma - LH$ and $\Gamma - HH$ direct gap transition were found to be respectively 0.7749 and 0.7896 eV which is in excellent agreement with the 8-band k.p estimation that gives respectively 0.7761 and 0.7897 eV for a tensile-strained Ge-VS layer with 0.13%. Finally, the modeled IRSE spectra with (red line) and without (dashed blue line) the incorporation of the direct band gap interband transitions is presented in Fig S3d. Additionally, a model based on a previous work [9] is shown (orange dashed line) and indicates the inaccuracy in dealing with the $LH$ and $HH$ to $\Gamma$ direct gap transition. Neglecting the direct band gap interband transition will underestimate the physical thickness of the Ge-VS and leads to an increase of the MSE from 1.512 to 2.145. To that end, the LH-HH modified optical parametrization of the Ge layer will be used in the remainder of this work and will serve to extract the GeSn buffer optical properties.

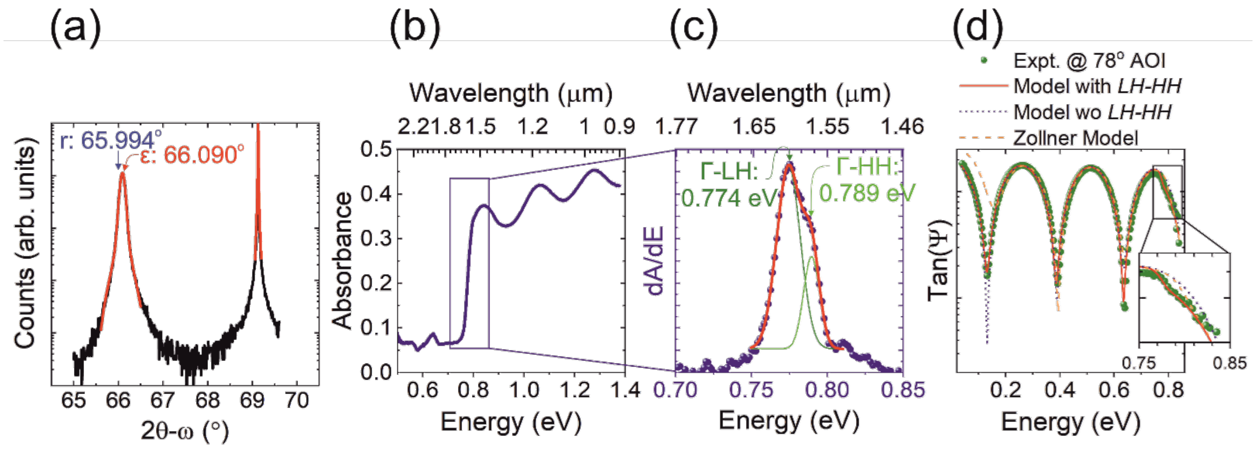


Figure S3: (a) $2\omega - \theta$ scans around the (004) X-ray diffraction order for the 0.13% tensile strained 650 nm Ge-VS layer. (b) Measured absorbance of the Ge-VS with an integrating sphere. The blue rectangle indicates the direct band gap region of the Ge layer. (c) Numerical estimation of the spectral derivative of the absorbance between 0.7 and 0.85 eV to highlight the effect of the $\Gamma - LH$ and $\Gamma - HH$ direct band gap transitions. The $\Gamma - LH$ and $\Gamma - HH$ direct band gap transitions were fitted with a gaussian distribution to estimate the energy transitions. (d) All the aforementioned characterizations are incorporated into the newly developed Ge IRSE optical model where the introduction of the LH and HH direct band transitions leads to a fit improvement as shown in the inset.

### S2.3. *Optical Modeling Strategy*

The buffer of the 1.1% tensile strained QW series (labelled as $V_1$, henceforth) is composed of three $\mathrm{Ge_{1-x}Sn_x}$ layers labelled #1, #2 and TL grown on top of the Ge-VS. Also, the three layers in the buffer have a gradually varying composition. RSM measurements around the asymmetrical (224) XRD reflection of the buffer sample ($V_1^{\mathrm{Buffer}}$) as well as each independently grown layer of the buffer ($V_1^{\#1}$, $V_1^{\#2}$, and $V_1^{\#3}$) are shown in Fig. S4. Fig. S4a highlights the symmetric (004) simple $2\omega - \theta$ scan where the contribution of each layer is shown with the arrows (#1, #2 and #3). To build a physically sound optical model for the buffer, different samples each having an individual GeSn layer grown on a Ge-VS layer (GeSn/Ge-VS/Si) were prepared with a Sn content and an epitaxial strain that matches the properties of each layer in the buffer. For instance, 1 sample ($V_1^{\#1}$) having 8.8% Sn content and -0.25 compressive strain (RSM map in Fig S4b) grown at 320°C was prepared and analyzed with IRSE. The same was done to extract the corresponding optical model of the layers #2 and #3. Additionally, the presence of interdiffusion at the GeSn/Ge and Ge/GeSn interfaces renders the analysis of graded layers more complicated. The presence of grading makes the optical model more tedious, but the following approach was used. In the current work, the GeSn buffer grading was first quantified with a combination of EDX (not shown here) and RSM

maps. First, the RSM map, shown in Fig.S4e of the complete buffer, proves that some grading is present, especially in the TL layer, due to the visible broadening in the TL layer. Second, EELS measurement for the buffer sample were undertaken (not shown here) and confirmed the composition broadening where the evolution of Sn and Ge contents in the buffer were analyzed. However, an absolute estimation of the Sn content from EELS profile was not possible due to calibration issues. Thus, combing the EELS spectra with the RSM maps can give a quantitative evaluation of the Sn grading inside the buffer, more specifically inside the TL layer. The following structural information is then used to include the effect of the buffer grading to the quantum well sample. This approximation has been verified with EELS profiles for all the studied quantum well. Graded layers are simulated in the VASE model by breaking the layer into n+1 sublayer. The thickness of the $i^{th}$ sublayer is defined as

$$d_i = \begin{cases} \dfrac{D}{2n} & ; i = 0, n \\ \dfrac{D}{n}; & i = 1 \dots n-1 \end{cases}$$

where D is the TL layer total thickness. For the linearly graded layer, the Sn content $x_i$ in the $i^{th}$ sublayer will be given by $x_i = \big((n-i)x_0 + ix_n\big)/n$ where $x_0$ and $x_n$ are the Sn content in the #2/TL and TL/sGe interfaces. Furthermore, due to the small gradient, this approach can be successful to estimate the effective dielectric function of the layer. Fig S5 shows the raw spectroscopic parameter ($\tan\Psi$ at 78° AOI) with the optical model for the buffer sample, and each constituent layer in the schematic model. Considering the effect of grading in the layer reduces the MSE from 10 to 2.5, which is a clear indication that the optical model encompasses the physical nature of the studied sample. The optical properties of the buffer layer are then fixed (only the thickness of the total buffer layer is changed) to reduce the correlation error between the different optical model parameters of each layer. Table 1 shows a detailed structural characterization for all the constituent's buffer layers in the studied $V_1$ series, where the Sn at. %, and the epitaxial strain $\varepsilon_{\parallel}$ are evaluated. Likewise, the thicknesses estimated from XTEM maps and IRSE modeling are given in Table 1.

Table 1: Structural information of the buffer layers used to build the optical model of V₁.

| param s / layer | $V_1^{\mathrm{Buffer}}$ | | | | $V_1^{\#1}$ | | | | $V_1^{\#2}$ | | | | $V_1^{TL}$ | | | |
|---|---|---|---|---|---|---|---|---|---|---|---|---|---|---|---|---|
| | Sn (%) | $\varepsilon_{\parallel}$ (%) | $d_i^a$ (nm) XTEM | $d_i^a$ (nm) IRSE | Sn (%) | $\varepsilon_{\parallel}$ (%) | $d_i^a$ (nm) XTEM | $d_i^a$ (nm) IRSE | Sn (%) | $\varepsilon_{\parallel}$ (%) | $d_i^a$ (nm) XTEM | $d_i^a$ (nm) IRSE | Sn (%) | $\varepsilon_{\parallel}$ (%) | $d_i^a$ (nm) XTEM | $d_i^a$ (nm) IRSE |
| Ge-VS | N.A. | 0.16 | 961 | 950 | N.A. | 0.15 | 965 | 970 | N.A. | 0.15 | 962 | 968 | N.A. | 0.15 | 963 | 972 |
| #1 | 8.3 | -0.26 | 140 | 141 | 8.7 | -0.30 | | | | | | | 7.0 | -0.12 | 225 | 230 |
| #2 | 10.3 | -0.46 | 133 | 126 | | | | | 10.2 | -0.45, -0.63 | 350 | 365 | | | | |
| #3 | 11.8 | -0.64 | 223 | 238 | | | | | | | | | 11.6 | -0.63 | 410 | 405 |
| RMS | | | 8.0± 0.5 | | | | 57.3± 5.4 | | | | 6.0 ±0.5 | | | | 4.5 ±1.0 | |

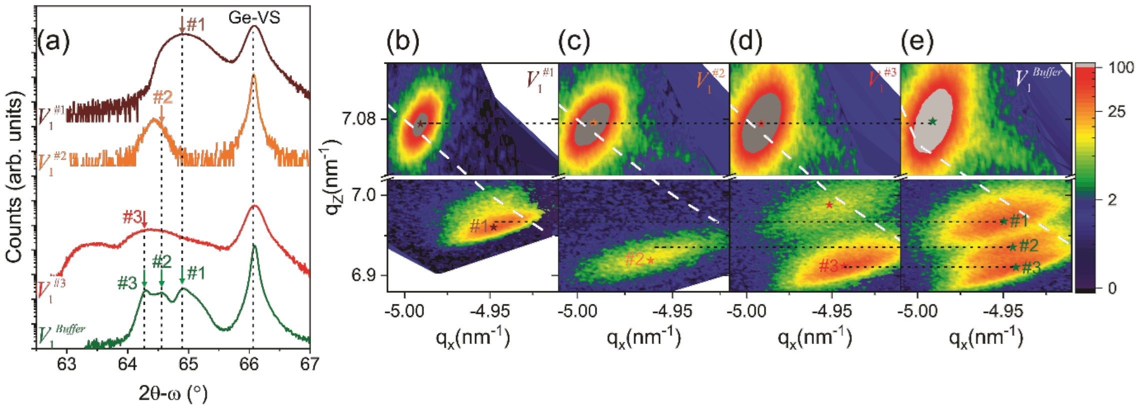


Figure S4: (a) $2\omega - \theta$ scans around the (004) X-ray diffraction order of the buffer sample $V_1^{\mathrm{Buffer}}$ and all the corresponding constituent layers, measured independently from epitaxially grown samples. The dashed lines represent the peak position of the corresponding buried layer within the buffer. The (224) RSM maps of the buffer (panel e) and each constituent layer (panel b for layer #1, panel c for layer #2, and panel d for layer #3) is acquired to quantify the Sn at.% as well as the compressive strain and compare the difference between the complete buffer and each layer to confirm the reliability of the corresponding samples to extract the correct optical properties. The dashed white line represents the relaxation line.

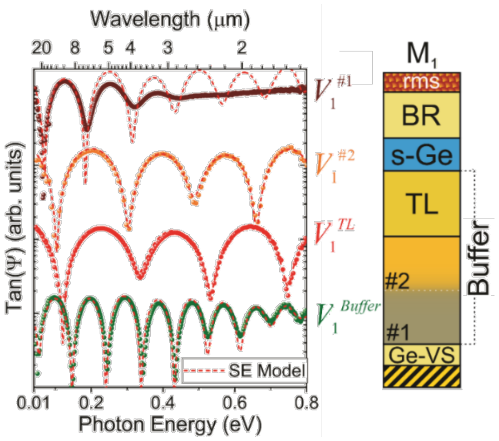


Figure S5: Approach to build the SE optical model for the buffer of the 1.1% tensile sGe QW. IRSE parameter (tan Ψ) for the different samples shown in Fig.S4 measured at 78°. The right-hand side sketch is a schematic of the stack used for the SE model based upon the low-resolution TEM image of Fig. 2a. The RMS layer was added to include the effect of surface overlayer and surface roughness.

## S3. Structural and optical characterization of s-Ge QWs

S3.1. *Ge QW at 1.1% tensile strain*

Three types of heterostructures series were investigated during this work (labelled as $V_1, V_2$ and $V_3$). Briefly, $V_1$ is a tensile strained Ge QW where the strain is estimated from HRXRD to be around 1.1%. $V_2$ is a multilayer system where the effect of the confinement is supressed by growing epitaxially the multilayer without the barrier (BR) layer. Finally, $V_3$ is a tensile-strained Ge QW where the strain reaches up to 1.65%. Asymmetric RSM map (Fig. S1b) measured along the (224) direction for each sample in the $V_1$ series highlights the contribution of each layer in the multi-stack, except the thin (below 12.5nm) s-Ge tensile strained layer, where more detailed analysis needs to be done as shown in section 1. The coherent growth of a s-Ge tensile strained layer with 1.1% strain was confirmed with HRRSM. Table 2 shows a detailed structural characterization for all the different QW with the variable thicknesses in the studied $V_1$ series, where the Sn at. %, and the epitaxial strain $\varepsilon_{||}$ are evaluated.

S3.2. *Uncapped Ge layer at 1.1% tensile strain*

Additionally, the second series $V_2$ aims into disregarding the effect of confinement by systematically growing a tensile-strained Ge layer with 1.1% tensile-strain without a BR layer. Buffer strain engineering is the path toward achieving this aim. The $V_2$ series is composed of 5 samples as shown in Fig. S6a and Table 3. Four of theses samples detail the buffer growth, which is fundamental for an exact IRSE analysis, while the remaining one is the sample of interest with the s-Ge layer grown on top of the TL layer, with a tensile strain of 1.1%. The samples in this series will be labeled as $V_2^i$ where $i$ is the grown layer(s) number(s). For example, $V_2^{\#2+3}$ is the sample where the layers #2 and #3 are grown on top of the Ge-VS and the layer #1, and so on. Having a systematic layer by layer growth will render the IRSE optical modelling more precise as, correlation uncertainties will be reduced. The schematic of the $V_2^{s-Ge}$ sample, shown in Fig. S7 constitutes the main optical model for the IRSE analysis. The presence of a defect free s-Ge layer is confirmed with a HRSTEM (not shown) and EELS profile line-scan of the Ge at. % where the top s-Ge layer is clearly visible. The thickness of the s-Ge is estimated to be 5.6 nm. The $2\theta - \omega$ XRD scans around the (004) X-ray diffraction order for the buffer layers as well as the s-Ge capping layer is presented in Fig. S6a. Additionally, the RSM (224) maps for the aforementioned samples are presented in Fig. S6b. The buried layer Sn at. % as well as the epitaxial strain are

extracted from the RSM map and are tabulated in Table 3. The buffer of the $V_2$ series is composed of three $Ge_{1-x}Sn_x$ layers (#1, #2 and #3, as indicated by the colored stars in Fig. S6b) with increasing Sn at.% ranging from 5 at.% to 8.8 at.%. Each sample is then independently characterized with IRSE to build the layer-by-layer optical model for the $V_2^{s-Ge}$ sample to obtain the corresponding dielectric function of the s-Ge layer. The results of the optical modelling are shown in Fig. S7 where the raw and modelled SE parameter $tan\,\Psi$ is shown for all the samples within the $V_2$ series at 78°.

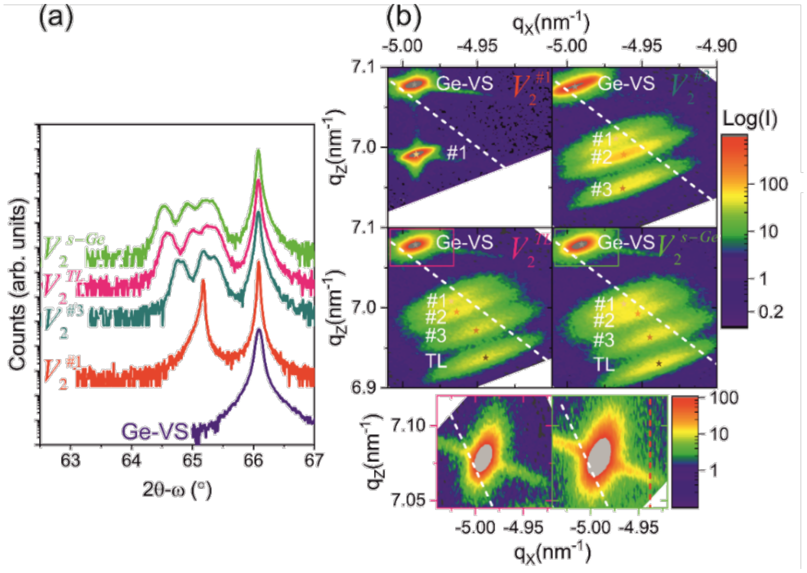


Figure S6: (a) $2\omega - \theta$ scans around the (004) X-ray diffraction order for the $V_2$ series samples. The arrows indicate the sequential layer by layer growth approach is highlighted. (b) RSM maps around the asymmetrical (224) reflection of the $V_2$ series samples in (a). The dashed white line is the relaxation line with regards to the Ge-VS layer. Each GeSn layer is indicated with its corresponding label as defined in the main text. The corresponding Sn at.% and epitaxial strain can thus be extracted from these maps. The corresponding values are shown in Table 3. The red (no s-Ge cap) and green (with s-Ge cap) insets are focused RSM maps around the Ge peak acquired with higher integration time in order to visualize the presence of the s-Ge cap layer. The red dashed line shows the theoretical position of a 1.1% tensile strained Ge cap layer, coherently grown to the TL.

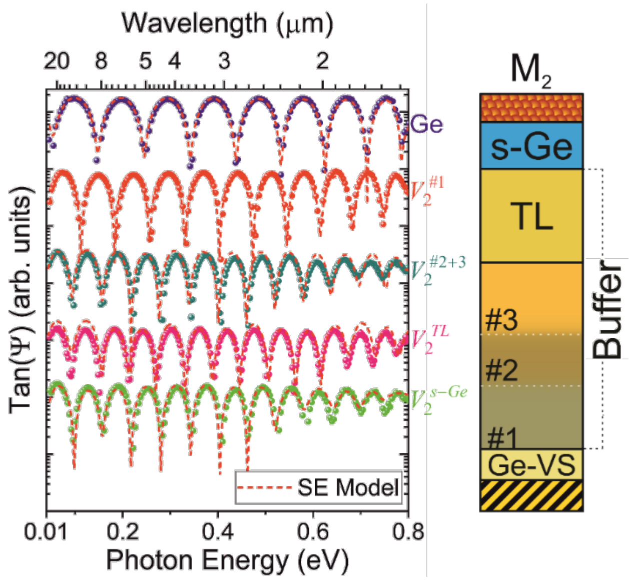


Figure S7: IRSE model of the $V_2$ series for all the constituent buffer layers, measured at 78°. The schematic shows the stack used to model the raw SE parameter.

S3.3. *Ge QW at 1.65% tensile strain*

The third series $V_3$ was fabricated in order to increase the tensile strain inside the Ge layer above 1.5% to achieve a higher LH confinement in the s-Ge QW. All the structural information concerning the $V_3$ series are shown in Table 4. $V_3^{s-Ge}$ is a 3.5 nm s-Ge QW with a tensile strain of 1.65 %. The tensile strain was estimated from RSM map by assuming a coherent growth, as shown in section S1. All the other samples are the layer-by-layer samples needed to build the SE optical model. It is important to indicate that the buffer has 2 additional layers with regards to the $V_2$ series. The reason behind this is to increase the Sn incorporation in the TL layer to reach above 15 at.% which would guarantee a tensile strain of around 1.7% inside the coherently-grown Ge layer. However, the Sn content at the TL layer was estimated with HRRSM to be 14.7 % which translates to a tensile strain of 1.65 %. Fig. S8 shows the different RSM maps for all the buffer layers as well as the QW sample. The sample labeling is similar to that of $V_2$ series. From Fig. S9, the different Sn content and epitaxial strain can be evaluated, as described in section 1, and the corresponding results are shown in Table 4. Finally, with the acquired knowledge of the structural properties, it becomes possible to build the optical model for all the buffer samples (from $V_3^{\#1}$ to $V_3^{TL}$), as shown in Fig. S9.

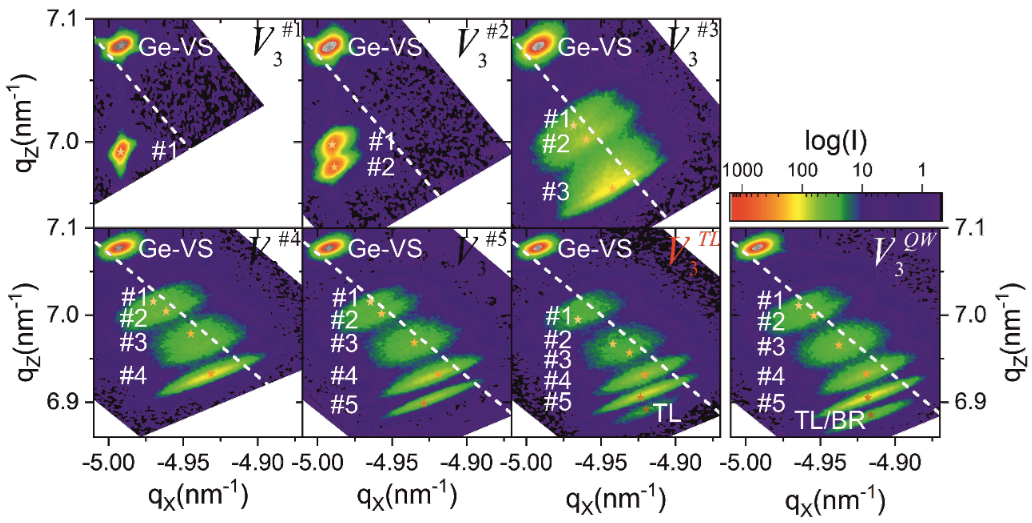


Figure S8: RSM maps around the asymmetrical (224) reflection of the $V_3$ series samples. From top left to bottom right: $V_3^{\#1} \rightarrow V_3^{QW}$. The stars indicate the highest detected intensity for each GeSn layer. The dashed white line is the relaxation line with regards to the Ge-VS layer. Each GeSn layer is indicated with its corresponding label as defined in the main text. The corresponding Sn at.% and epitaxial strain are shown in Table 4.

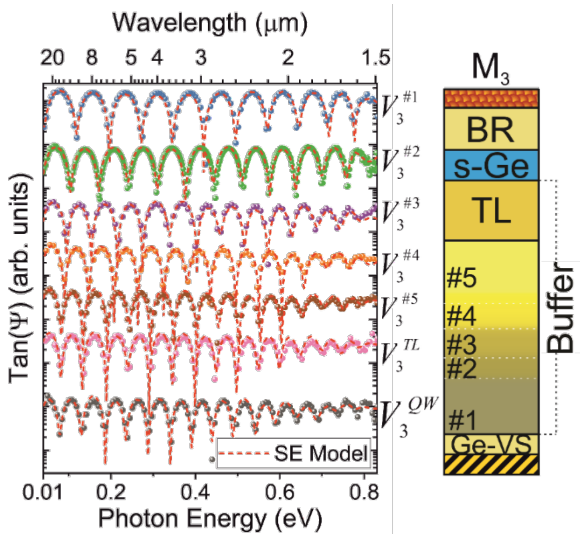


Figure S9: IRSE model of the $V_3$ series for all the constituent buffer layers, measured at 78°. The schematic on the right shows the stack used to model the raw SE parameter.

Table 2: 1.1% tensile strain Ge QW $V_1$ series structural characterization

| params / layer | $V_1^{Ge-VS}$ | | | | $V_1^{\text{Buffer}}$ | | | | $V_1^{45\ min}$ | | | | $V_1^{25\ min}$ | | | | $V_1^{15\ min}$ | | | |
|---|---|---|---|---|---|---|---|---|---|---|---|---|---|---|---|---|---|---|---|---|
| | Sn (%) | $\varepsilon_\parallel$ (%) | $d_i$ (nm) XTEM | $d_i$ (nm) IRSE | Sn (%) | $\varepsilon_\parallel$ (%) | $d_i$ $(nm)$ XTEM | $d_i$ $(nm)$ IRSE | Sn (%) | $\varepsilon_\parallel$ (%) | $d_i$ $(nm)$ XTEM | $d_i$ $(nm)$ IRSE | Sn (%) | $\varepsilon_\parallel$ (%) | $d_i$ $(nm)$ XTEM | $d_i$ $(nm)$ IRSE | Sn (%) | $\varepsilon_\parallel$ (%) | $d_i$ (nm) XTEM | $d_i$ (nm) IRSE [b] |
| Ge-VS | 0 | 0.08 | 950 | 932 | 0 | 0.16 | 961 | 955 | 0 | 0.15 | 961 | 950 | 0 | 0.15 | 922 | 950 | 0 | 0.14 | 916 | 940 |
| #1 | | | | | 8.3 | -0.26 | 140 | 132 | 8.6 | -0.33 | 117 | 110 | 8.3 | -0.17 | 124 | 120 | 8.8 | -0.14 | 83 | 75 |
| #2 | | | | | 10.3 | -0.46 | 133 | 125 | 10.8 | -0.55 | 118 | 120 | 10.2 | -0.44 | 128 | 130 | 10.1 | -0.43 | 133 | 120 |
| TL | | | | | 11.8 | -0.64 | 223 | 235 | 11.9 | -0.68 | 200 | 210 | 11.8 | -0.64 | 207 | 200 | 11.1 | -0.48 | 221 | 230 |
| s-Ge | | | | | | | | | | 1.1 | 12.5 | 13 | | 1.1 | 10.5 | 11 | | 1.1 | 7.5 | 8.0 |
| BR | | | | | | | | | 13.4 | -0.94 | 34 | 30 | 13.2 | -0.85 | 39 | 40 | 12.3 | -0.63 | 72 | 75 |
| RMS [a] | | | 4.7<br>±0.8 | | | | 8±1 | | | | 9.0<br>±0.9 | 10 | | | 15<br>±5 | 11 | | | 7.5<br>±1.5 | 8.5 |

[a] The RMS is measured with a 20x20 $\mu m^2$AFM maps.

[b] The error estimation of the IRSE is ±4nm.

Table 2: ctd.

| params / layer | $V_1^{8\ min}$ | | | | $V_1^{5\ min}$ | | | | $V_1^{2\ min}$ | | | |
|---|---|---|---|---|---|---|---|---|---|---|---|---|
| | Sn (%) | $\varepsilon_\parallel$ (%) | $d_i$ $(nm)$ XTEM | $d_i$ $(nm)$ IRSE | Sn (%) | $\varepsilon_\parallel$ (%) | $d_i$ $(nm)$ XTEM | $d_i$ $(nm)$ IRSE | Sn (%) | $\varepsilon_\parallel$ (%) | $d_i$ $(nm)$ XTEM | $d_i$ $(nm)$ IRSE |
| Ge-VS | 0 | 0.14 | 932 | 940 | 0 | 0.17 | 961 | 960 | 0 | 0.16 | 961 | 960 |
| #1 | 8.5 | -0.24 | 79 | 80 | 7.8 | -0.17 | 121 | 120 | 8.1 | -0.30 | 138 | 140 |
| #2 | 10.4 | -0.56 | 139 | 140 | 10.1 | -0.49 | 123 | 130 | 9.9 | -0.45 | 136 | 135 |
| TL | 11.4 | -0.69 | 232 | 240 | 11.3 | -0.61 | 209 | 210 | 11.4 | -0.65 | 235 | 230 |
| s-Ge | | 1.1 | 3.5 | 4 | | 1.1 | 2.7 | 3 | | 1.1 | 1.5 | 2 |
| BR | 12.4 | -0.80 | 46 | 50 | 12.2 | -0.74 | 43 | 50 | 12.5 | -0.76 | 48 | 50 |
| RMS | | | 5.3<br>±0.8 | 6 | | | 7.2<br>±1.9 | 8 | | | 7.5<br>±1.1 | 6.5 |

Table 3: Uncapped Ge layer $V_2$ series structural information

| params / layer | $V_2^{Ge-VS}$ | | | | $V_2^{\#1}$ | | | | $V_2^{\#2+3}$ | | | | $V_2^{TL}$ | | | | $V_2^{s-Ge}$ | | | |
|---|---|---|---|---|---|---|---|---|---|---|---|---|---|---|---|---|---|---|---|---|
| | Sn (%) | $\varepsilon_\parallel$ (%) | $d_i^a$ (nm) XTEM | $d_i^a$ (nm) IRSE | Sn (%) | $\varepsilon_\parallel$ (%) | $d_i$ $(nm)$ XTEM | $d_i$ $(nm)$ IRSE | Sn (%) | $\varepsilon_\parallel$ (%) | $d_i$ $(nm)$ XTEM | $d_i$ $(nm)$ IRSE | Sn (%) | $\varepsilon_\parallel$ (%) | $d_i^a$ (nm) XTEM | $d_i^a$ (nm) IRSE | Sn (%) | $\varepsilon_\parallel$ (%) | $d_i^a$ (nm) EELS | $d_i^a$ (nm) IRSE |
| Ge-VS | 0 | 0.14 | | 1628 | 0 | 0.14 | | 1675 | 0 | 0.08 | | 1680 | 0 | 0.15 | | 1630 | 0 | 0.16 | 1650 | 1628 |
| #1 | | | | | 4.7 | -0.54 | | 250 | 5.0 | -0.13 | | 195 | 5.1 | -0.14 | | 205 | 5.6 | -0.11 | 201 | 200 |
| #2 | | | | | | | | | 6.3 | -0.22 | | 125 | 6.0 | -0.21 | | 135 | 6.8 | -0.10 | 138 | 140 |
| #3 | | | | | | | | | 8.5 | -0.56 | | 155 | 8.0 | -0.24 | | 145 | 8.8 | -0.24 | 149 | 150 |
| TL | | | | | | | | | | | | | 10.1 | -0.44 | | 120 | 10.9 | -0.43 | 123 | 125 |
| s-Ge | | | | | | | | | | | | | | | | | | 1.1 | 4.5 | 5.12 |
| RMS [a] | | | 1.0<br>±0.1 | 1.5<br>±1.0 | | | 5.4<br>±1.5 | 6±1 | | | 8.1<br>±0.3 | 7.5<br>±0.5 | | | 9.5<br>±1.4 | 10<br>±1 | | | 8.6<br>±0.3 | 9<br>±1 |

[a] The RMS is measured with a 20x20 $\mu m^2$AFM maps.

Table 4: 1.65% tensile strain Ge QW $V_3$ series RSM structural information

| params / layer | $V_3^{Ge-VS}$ | | | | $V_3^{\#1}$ | | | | $V_3^{\#2}$ | | | | $V_3^{\#3}$ | | | | $V_3^{\#4}$ | | | |
|---|---|---|---|---|---|---|---|---|---|---|---|---|---|---|---|---|---|---|---|---|
| | Sn (%) | $\varepsilon_{\parallel}$ (%) | $d_i^a$ (nm) | | Sn (%) | $\varepsilon_{\parallel}$ (%) | $d_i$ $(nm)$ | | Sn (%) | $\varepsilon_{\parallel}$ (%) | $d_i$ $(nm)$ | | Sn (%) | $\varepsilon_{\parallel}$ (%) | $d_i$ $(nm)$ | | Sn (%) | $\varepsilon_{\parallel}$ (%) | $d_i$ $(nm)$ | |
| | | | XTEM | IRSE | | | EDS | IRSE | | | EDS | IRSE | | | XTEM | IRSE | | | XTEM | IRSE[b] |
| Ge-VS | 0 | 0.15 | 1628 | 1650 | 0 | 0.16 | 1630 | 1638 | 0 | 0.14 | | 1640 | 0 | 0.15 | 1623 | 1640 | 0 | 0.12 | 1675 | 1670 |
| #1 | | | | | 4.6 | -0.54 | | 190 | 4.3 | -0.47 | | 190 | 4.7 | -0.10 | 200 | 210 | 4.5 | -0.10 | 200 | 210 |
| #2 | | | | | | | | | 4.7 | -0.60 | | 150 | 5.8 | -0.10 | 161 | 165 | 5.6 | -0.09 | 161 | 155 |
| #3 | | | | | | | | | | | | | 8.9 | -0.21 | 320 | 325 | 9.2 | -0.18 | 327 | 330 |
| #4 | | | | | | | | | | | | | | | | | 11.3 | -0.34 | 263 | 260 |
| #5 | | | | | | | | | | | | | | | | | | | | |
| TL | | | | | | | | | | | | | | | | | | | | |
| s-Ge | | | | | | | | | | | | | | | | | | | | |
| BR | | | | | | | | | | | | | | | | | | | | |
| RMS [a] | | | 1.0 ±0.1 | 1.0 ±0.5 | | | 6 ±2 | 5 ±1 | | | 8 ±2 | 7 ±2 | | | 9.5 ±0.5 | 9 ±1 | | | 8.3 ±1.6 | 8 ±2 |

[a] The RMS is measured with a 20x20 μm$^2$AFM maps.

[b] The thickness error estimation of the IRSE is ±2nm.

Table 4: ctd.

| params / layer | $V_3^{\#5}$ | | | | $V_3^{TL}$ | | | | $V_3^{QW}$ | | | |
|---|---|---|---|---|---|---|---|---|---|---|---|---|
| | Sn (%) | $\varepsilon_{\parallel}$ (%) | $d_i^a$ (nm) | | Sn (%) | $\varepsilon_{\parallel}$ (%) | $d_i$ $(nm)$ | | Sn (%) | $\varepsilon_{\parallel}$ (%) | $d_i$ $(nm)$ | |
| | | | XTEM | IRSE | | | XTEM | IRSE | | | EELS | IRSE |
| Ge-VS | 0 | 0.14 | 1685 | 1690 | 0 | 0.14 | 1620 | 1630 | 0 | 0.14 | 1556 | 1600 |
| #1 | 4.8 | -0.05 | 180 | 185 | 5.8 | -0.10 | 200 | 205 | 5.1 | -0.10 | 180 | 185 |
| #2 | 6.0 | -0.10 | 150 | 145 | 8.7 | -0.17 | 161 | 160 | 8.3 | -0.10 | 151 | 150 |
| #3 | 9.0 | -0.10 | 300 | 310 | 9.9 | -0.12 | 320 | 319 | 9.1 | -0.14 | 346 | 350 |
| #4 | 11.9 | -0.25 | 275 | 280 | 11.9 | -0.22 | 263 | 260 | 12.0 | -0.19 | 212 | 215 |
| #5 | 13.1 | -0.54 | 450 | 455 | 13.0 | -0.44 | 160 | 158 | 13.5 | -0.40 | 158 | 160 |
| TL | | | | | 14.1 | -0.52 | 48 | 50 | 14.7 | -0.54 | 48 | 50 |
| s-Ge | | | | | | | | | 0 | 1.67 | 3.5 | 3.65 |
| BR | | | | | | | | | 14.7 | -0.54 | 15 | 18 |
| RMS | | | 10.3 ±1.4 | 9 ±2 | | | 10.6 ±1.5 | 8 ±2 | | | 12.3 ±1.2 | 9 ±1 |

## S4. Theoretical Simulation

S4.1. *Eight-band **k·p** GeSn Parametrization*

Table 5 contains all the material parameters that were used in the 8-band $k \cdot p$ simulations. Values for the lattice constants correspond to a temperature of 300 K.

Table 5: Material parameters of Ge$_{1-x}$Sn$_x$ for the $k \cdot p$ model

| | Ge | Sn | Ge$_{1-x}$Sn$_x$ bowing |
|---|---|---|---|
| Lattice constant | | | |
| $a_0$ (Å) | 5.657956[a] | 6.489417[b] | -0.083[c] |
| CB effective mass | | | |
| $m_{c\Gamma}$ ($m_0$) | 0.0383[d] | -0.058[e] | |
| Band gaps | | | |
| $E^0_{\mathrm{g}\Gamma}$ (eV) | 0.8981[d] | -0.39[f] | |
| $E^0_{\mathrm{gL}}$ (eV) | 0.785[d] | 0.100[c] | |
| $\alpha_\Gamma$ ($10^{-4}$ eV/K) | 6.842[d] | -0.794[f] | |
| $\alpha_{\mathrm{L}}$ ($10^{-4}$ eV/K) | 4.561[d] | - | |
| $\beta_\Gamma$ (K) | 398[d] | 11[f] | |
| $\beta_{\mathrm{L}}$ (K) | 210[d] | - | |
| $\Delta$ (eV) | 0.289[c] | 0.600[c] | -0.1[c] |
| Average valence band | | | |
| $E_{v,\mathrm{avg}}$ (eV) | 0 | 0.69[g] | |
| Elastic constants | | | |
| $c_{11}$ (GPa) | 128.53[d] | 69.00[g] | |
| $c_{12}$ (GPa) | 48.28[d] | 29.30[g] | |
| $c_{44}$ (GPa) | 66.80[d] | 36.20[g] | |
| Deformation potentials † | | | |
| $a_{c\Gamma}$ (eV) | -10.41[d] | -6.00[g] | |
| $a_{cL}$ (eV) | -1.54[d] | -2.14[g] | |
| $a_v$ (eV) | 1.24[d] | 1.58[g] | |
| $b$ (eV) | -2.86[d] | -2.7[g] | |
| $d$ (eV) | -5.28[d] | -4.1[b] | |
| Luttinger parameters | | | |
| $\gamma_1$ | 13.37[d] | 29.2108[h] * | 20.3391[h] |
| $\gamma_2$ | 4.23[d] | 12.2413[h] * | 9.6609[h] |
| $\gamma_3$ | 5.68[d] | 13.7387[h] * | 9.8187[h] |
| $\kappa$ | 3.41[e] | -11.84[e] | |
| $g$ | -2.86[e] | 84.4[e] | |

†: The convention $a = a_c - a_v$ is used.

*: Values for Ge$_{0.8}$Sn$_{0.2}$.

[a]Ref.10 [b]Ref.11, [c]Ref. 12, [d]Ref. 13, [e]Ref. 14, [f]Ref. 15, [g]Ref. 16, [h]Ref. 17

S4.2. *Magnetic Field incorporation in 8-band* $\boldsymbol{k{\cdot}p}$

A uniform magnetic field with orientation $(\theta, \varphi)$ is included in the $k \cdot p$ matrix by writing the vector potential $\mathbf{A}$ as

$$\mathbf{A} = (B/2)[(-y\cos\theta + 2z\sin\theta\sin\varphi)\hat{\mathbf{x}} + (x\cos\theta - 2z\sin\theta\cos\varphi)\hat{\mathbf{y}}]$$

and by writing the Hamiltonian in terms of mechanical wavenumber $\mathbf{K} = \mathbf{k} + e\mathbf{A}/\hbar$, where $e$ is the elementary charge. The contribution of the free electron spin was added to the Hamiltonian [18] $H_B = 1/2\, g_0 \mu_B \boldsymbol{\sigma} \cdot \mathbf{B}$, with $g_0$ the free electron g-factor, $\mu_B$ the Bohr magneton and $\boldsymbol{\sigma}$ the vector of Pauli matrices. For perpendicular-to-plane fields ($\theta = 0$), we define the annihilation and creation operators $a = \lambda/\sqrt{2}\,(K_x - iK_y)$, $a^\dagger = \lambda/\sqrt{2}\,(K_x + iK_y)$, where $\lambda = \sqrt{\hbar/eB}$ is the magnetic length, and the Hamiltonian is written in axial approximation in terms of $a$ and $a^\dagger$ as in Refs. [19,20]. The ladder operators act on Landau oscillators $|n\rangle$ in the usual way: $a|n\rangle = \sqrt{n}|n-1\rangle$, $a^\dagger|n\rangle = \sqrt{n+1}|n+1\rangle$ and $a^\dagger a|n\rangle = n|n\rangle$. We then proceed to block diagonalize the Hamiltonian, with each block corresponding to a given Landau number $n$. [21] On the other hand, for in-plane magnetic fields ($\theta = \pi/2$), we diagonalize the $k \cdot p$ matrix as in the zero-field subband problem. However, to ensure gauge invariance of the energy dispersion, we choose the origin of the $z$-axis so that $\langle z \rangle = 0$. This results in the quantum numbers $k_x$ and $k_y$ to become equivalent to $\langle K_x \rangle$ and $\langle K_y \rangle$ respectively, which are gauge-independent quantities. A similar procedure was used in to ensure gauge-invariance. [22] Finally, effective $g$-factors were calculated in the weak-field regime ($B \sim 10^{-4}$ T), for which the Zeeman splitting between opposite spins remains linear.

S4.3. *Light hole-heavy hole mixing in highly tensile strained Ge QWs*

In the limit of highly strain relaxed GeSn barriers, a significant amount of tensile strain in Ge results in the light hole ground state (LH1) to be above the heavy hole continuum. The energy gap between LH1 and the continuum can be tuned by changing the Ge quantum well thickness. Fig. S10a shows how this energy gap affects light hole-heavy hole mixing in LH1 on a range of wavevectors in reciprocal space. The amplitude squared of the spinor component associated with heavy holes (HH contribution) vanishes at zero in-plane wavevector ($k_\parallel = 0$) and increases with $k_\parallel$. A HH contribution of 1 corresponds to a pure heavy hole subband. The increase rate of HH contribution is lower for thicker wells, consequence of a larger energy gap and a smaller wavefunction overlap between LH1 and the continuum. Fig S10b shows comparative calculations

in a Ge/SiGe heterostructure, where the Ge quantum well is 12.5 nm thick and compressively strained between relaxed SiGe barriers. In contrast to tensile strained Ge, LH1 is separated from the band gap by a few heavy hole subbands (three for 12.5 nm well), but most notably, its HH contribution reaches significantly higher values. Consequently, the light hole-like valence band edge of highly tensile strained Ge quantum wells is subject to reduced amounts of mixing compared to light hole subbands in a compressively strained Ge quantum well.

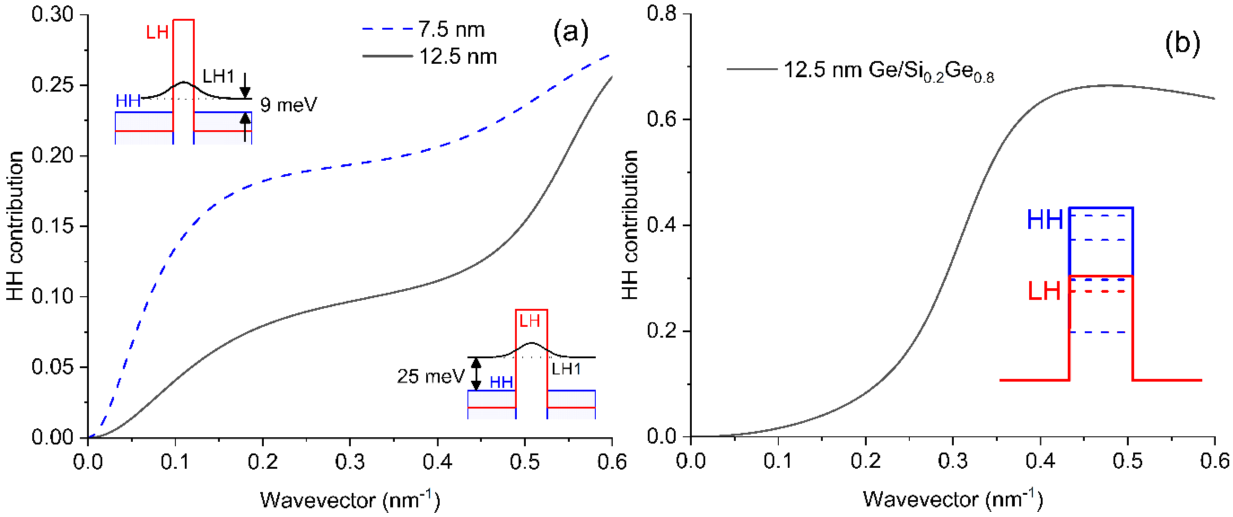


Figure S10: $k \cdot p$ band structure calculations of light hole-heavy hole mixing. (a) Tensile strained Ge quantum well between $Ge_{0.87}Sn_{0.13}$ barriers with -0.125% residual strain. (b) Compressively strained Ge quantum well between relaxed $Si_{0.2}Ge_{0.8}$ barriers. Insets show real-space band alignments with subband energy levels (dashed lines) and light hole envelope function (not shown in b panel).

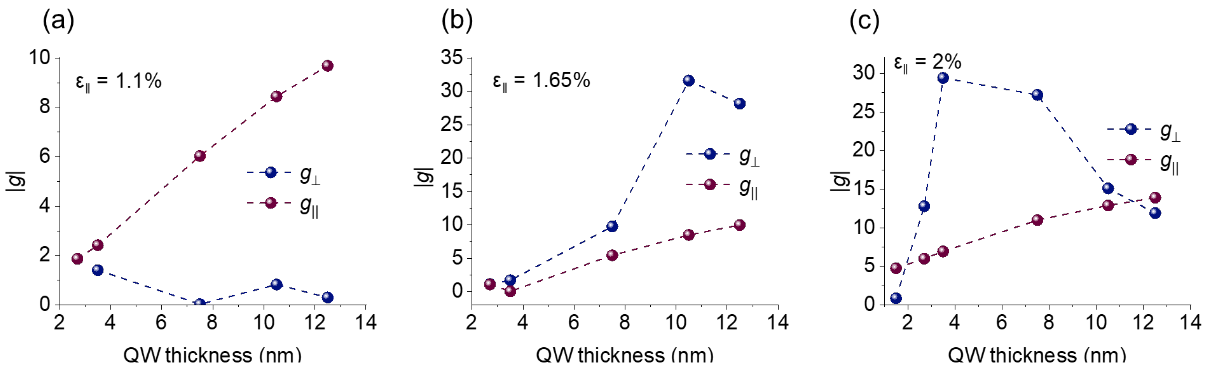


Figure S11: LH $g$-factor as a function of the Ge/GeSn QW thickness at a tensile strain of 1.1% (a), 1.65% (b), and 2% (c) under in-plane ($g_{\|}$) and out-of-plane ($g_{\perp}$) field configurations.

**S5. References**


1. Xu, C., Senaratne, C. L., Culbertson, R. J., Kouvetakis, J. & Menéndez, J. Deviations from Vegard's law in semiconductor thin films measured with X-ray diffraction and Rutherford backscattering: The Ge1-ySnyand Ge1-xSixcases. *J. Appl. Phys.* **122**, 0–10 (2017).

2. McSkimin, H. J. Measurement of Elastic Constants at Low Temperatures by Means of Ultrasonic Waves–Data for Silicon and Germanium Single Crystals, and for Fused Silica. *J. Appl. Phys.* **24**, 988 (2004).

3. Kouvetakis, J., Menendez, J. & Chizmeshya, A. V. G. Tin-Based Group IV Semiconductors: New Platforms for Opto- and Microelectronics on Silicon. *Annu. Rev. Mater. Res.* **36**, 497–554 (2006).

4. Gencarelli, F. *et al.* Crystalline Properties and Strain Relaxation Mechanism of CVD Grown GeSn. *ECS J. Solid State Sci. Technol.* **2**, P134–P137 (2013).

5. Tapfer, L. & Ploog, K. X-ray interference in ultrathin epitaxial layers: A versatile method for the structural analysis of single quantum wells and heterointerfaces. *Phys. Rev. B* **40**, 9802–9810 (1989).

6. Tapfer, L., Ospelt, M. & von Känel, H. Monolayer resolution by means of x-ray interference in semiconductor heterostructures. *J. Appl. Phys.* **67**, 1298–1301 (1990).

7. Clavel, M. *et al.* Heterogeneously-grown tunable tensile strained germanium on silicon for photonic devices. *ACS Appl. Mater. Interfaces* **7**, 26470–26481 (2015).

8. Clavel, M., Goley, P., Jain, N., Zhu, Y. & Hudait, M. K. Strain-engineered biaxial tensile epitaxial germanium for high-performance Ge/InGaAs tunnel field-effect transistors. *IEEE J. Electron Devices Soc.* **3**, 184–193 (2015).

9. Nunley, T. N. *et al.* Optical constants of germanium and thermally grown germanium dioxide from 0.5 to 6.6eV via a multisample ellipsometry investigation. *J. Vac. Sci. Technol. B, Nanotechnol. Microelectron. Mater. Process. Meas. Phenom.* **34**, 061205 (2016).

10. Reeber, R. R. & Wang, K. Thermal expansion and lattice parameters of group IV

semiconductors. *Mater. Chem. Phys.* **46**, 259–264 (1996).

11. *Semiconductors Group IV Elements and III-V Compounds*. (Springer-Verlag Berlin Heidelberg, 1991).

12. Polak, M. P., Scharoch, P. & Kudrawiec, R. The electronic band structure of Ge1-xSnx in the full composition range: Indirect, direct, and inverted gaps regimes, band offsets, and the Burstein-Moss effect. *J. Phys. D Appl. Phys.* **50**, 5103 (2017).

13. Paul, D. J. 8-band k·p modelling of mid-infrared intersubband absorption in Ge quantum wells. *J. Appl. Phys.* **120**, (2016).

14. Lawaetz, P. Valence-band parameters in cubic semiconductors. *Phys. Rev. B* **4**, 3460–3467 (1971).

15. Bertrand, M. *et al.* Experimental Calibration of Sn-Related Varshni Parameters for High Sn Content GeSn Layers. *Ann. Phys.* **1800396**, 1–6 (2019).

16. Chang, G., Chang, S. & Chuang, S. L. Multiple-Quantum-Well Lasers. *IEEE J. quantum Electron.* **46**, 1813 (2010).

17. Lu Low, K., Yang, Y., Han, G., Fan, W. & Yeo, Y. C. Electronic band structure and effective mass parameters of Ge 1-xSnx alloys. *J. Appl. Phys.* **112**, 3715 (2012).

18. Eissfeller, T. & Vogl, P. Real-space multiband envelope-function approach without spurious solutions. *Phys. Rev. B* **84**, 195122 (2011).

19. Winkler, R., Merkler, M., Darnhofer, T. & Rössler, U. Theory for the cyclotron resonance of holes in strained asymmetric Ge-SiGe quantum wells. *Phys. Rev. B - Condens. Matter Mater. Phys.* **53**, 10858–10865 (1996).

20. Luttinger, J. M. Quantum Theory of Cyclotron Resonance in Semiconductors : General Theory. *Phys. Rev.* **96**, 529–530 (1954).

21. Winkler, R. *Spin Orbit Coupling Effects in Two-Dimensional Electron and Hole Systems*. (Springer, 2003). doi:10.1007/b13586.

22. Stano, P. *et al.* Orbital effects of a strong in-plane magnetic field on a gate-defined quantum dot. *Phys. Rev. B* **99**, 085308 (2019).
